# Supplementary material for: Secure and Verifiable Data Collaboration with Low-Cost Zero-Knowledge Proofs
Source: arXiv:2311.15310 source file (2023-11-26)
Supplement: Supplementary file 1 [file sec-appendix.tex]

\section{Appendix} \label{sec:appendix}

\subsection{Preliminaries Extension} \label{appendix:pre}

% \needcheck{May put detailed building-block algorithms here for completeness. }
%
% \needcheck{Move the constructions of batch verification here.}

\textbf{$\Sigma$-protocol for proof of squares $(( \textbf{x}, \textbf{r}_1, \textbf{r}_2), (\textbf{y}_1, \textbf{y}_2))$.}
% The first ZKP protocol is the $\Sigma$-protocol~\cite{camenisch1997proof}. Here we describe the constructions for proof of square $((x_i, r_{i1}, r_{i2})_{i=1}^k,(y_{i1}, y_{i2})_{i=1}^k)$ and proof of relation.
Denote $g, h \in \mathbb{G}$ the independent group elements. Given secrets $\textbf{x}, \textbf{r}_1, \textbf{r}_2 \in \mathbb{Z}_p^k$ and commitments $(\textbf{y}_{1}, \textbf{y}_{2}) = (g^{\textbf{x}} h^{\textbf{r}_{1}}, g^{\textbf{x}^2} h^{\textbf{r}_{2}})$, i.e.\ $y_{1i} = g^{x_i} h^{r_{1i}}$ and $y_{2i} = g^{x_i^2} h^{r_{2i}}$ for $i \in [1, k]$, the prover uses the function $\mathsf{GenPrfSq}()$ in Algorithm~\ref{alg:gen_prf_sq} to generate a proof $\pi$ that the secret in $y_{2i}$ is the square of the secret in $y_{1i}$ for every $i$. The verifies uses the function $\mathsf{VerPrfSq}()$ in Algorithm~\ref{alg:ver_prf_sq} to verify this proof based on $(\textbf{y}_{1}, \textbf{y}_{2})$.
%
% For $i = 1, \dots, k$, let $y_{1i} = g^{x_i} h^{r_{1i}}$ and $y_{2i} = g^{x_i^2} h^{r_{2i}}$ be the commitments, where $x_i,r_{1i},r_{2i} \in \mathbb{Z}_p$ are the secrets. To handle the square in power, we can rewrite $y_{i2} = y_{i1}^x h^{r_{i2} - r_{i1} x_i}$. 
% Then, the function $\mathsf{GenPrfSq}()$ in Algorithm~\ref{alg:gen_prf_sq} generates a proof $\pi$ that $(\textbf{y}_{1}, \textbf{y}_{2})$ is of the form $(g^{\textbf{x}} h^{\textbf{r}_{1}}, g^{\textbf{x}^2} h^{\textbf{r}_{2}})$ for some $\textbf{x}, \textbf{r}_{1}, \textbf{r}_{2} \in \mathbb{Z}_p^k$, which are held by the prover. Similarly, the function $\mathsf{VerPrfSq}()$ in Algorithm~\ref{alg:ver_prf_sq} verifies this proof based on $(\textbf{y}_{1}, \textbf{y}_{2})$. %
In Algorithm~\ref{alg:ver_prf_sq}, the random numbers $\alpha_i, \beta_i$ are used for batch verification of multiple equalities: $g^{s_{1i}} h^{s_{2i}} y_{1i}^c == t_{1i}$, $h^{s_{3i}} y_{1i}^{s_{1i}} y_{2i}^{c} == t_{2i}$ for $i \in [1,k]$.
Batch-verifying these equalities saves cost by a factor of $O(\log(k))$.

% $\mathsf{VerPrfSq}()$ uses batch verification to check equalities of multiple pairs of group elements, which saves cost by a factor of $O(\log(k))$. \needcheck{(need to change the presentation to make it different from Section 2).}

\vspace{1mm} \noindent
\textbf{$\Sigma$-protocol for proof of relation $((r, \textbf{v}^*, \textbf{s}),(z, \textbf{e}, \textbf{o}))$.} Given independent group elements $g, q, h_0, \dots, h_k \in \mathbb{G}$, the $\Sigma$-protocol to prove and verify that $z = g^r$, $e_i = g^{v_i} h_i^r$ $(i \in [0,k])$, $o_i = g^{v_i} q^{s_i}$ $(i \in [1,k])$, where $v^* = (v_0, \dots, v_k)$, is the pair of functions $\mathsf{GenPrfWf}()$ and $\mathsf{VerPrfWf}()$. The function $\mathsf{GenPrfWf}()$ in Algorithm \ref{alg:gen_prf_wf} generates a proof $\pi$ that $(z, \textbf{e}, \textbf{o})$ is of the form $(g^r, g^{\textbf{v}^*} \textbf{h}^r, g^{\textbf{v}} q^{\textbf{s}})$, where $\textbf{v} = (v_1, \dots, v_k)$. The function $\mathsf{VerPrfWf}()$ in Algorithm \ref{alg:ver_prf_wf} verifies this proof. Again, we use batch verification to verify multiple equalities: $u == g^w z^c$, $t_i == g^{y_i} h_i^y e_i^c$ $(i \in [0,k])$, $t_i^* == g^{y_i} q^{y_i'} o_i^c$ $(i \in [1,k])$.

\begin{algorithm}[t]
  \caption{$\mathsf{GenPrfSq}(g, h, \textbf{y}_1, \textbf{y}_2, \textbf{x}, \textbf{r}_1, \textbf{r}_2)$}
  \label{alg:gen_prf_sq}
%\hspace*{\algorithmicindent} 
  \begin{algorithmic}
  %\hspace*{\algorithmicindent} 
    \STATE Randomly sample $\textbf{v}_{1}, \textbf{v}_{2}, \textbf{v}_{3} \in \mathbb{Z}_p^k$.
    \STATE Compute $t_{1i} = g^{v_{1i}} h^{v_{2i}}$, $t_{2i} = y_{1i}^{v_{1i}} h^{v_{3i}}$ for $i \in [1, k]$.
    \STATE Compute $c = H(g, h, \textbf{y}_1, \textbf{y}_2, \textbf{t}_1, \textbf{t}_2)$.
    \STATE Compute $\textbf{s}_1 = \textbf{v}_1 - c \textbf{x}_1$, $\textbf{s}_{2} = \textbf{v}_{2} - c \textbf{r}_{1}$, and $\textbf{s}_{3} = \textbf{v}_{3} - c (\textbf{r}_{2} - \textbf{r}_{1} \circ \textbf{x})$.
    % \FOR{$i = 1, \cdots, k$}
    %     \STATE Compute $s_{i1} = v_{i1} - c x_{i1}$, $s_{i2} = v_{i2} - c r_{i1}$, $s_{i3} = v_{i3} - c (r_{i2} - r_{i1} x_i)$.
    % \ENDFOR
    \RETURN $\pi = (\textbf{t}_{1}, \textbf{t}_{2}, \textbf{s}_{1}, \textbf{s}_{2},\textbf{s}_{3})$.
\end{algorithmic}
\end{algorithm}

\begin{algorithm}[t]
  \caption{$\mathsf{VerPrfSq}(g, h, \textbf{y}_1, \textbf{y}_2, \pi)$}
  \label{alg:ver_prf_sq}
%\hspace*{\algorithmicindent} 
  \begin{algorithmic}
%\hspace*{\algorithmicindent} 
\STATE Unravel $\pi = (\textbf{t}_{1}, \textbf{t}_{2}, \textbf{s}_{1}, \textbf{s}_{2},\textbf{s}_{3})$.
\STATE Randomly sample $\alpha_i, \beta_i \in \mathbb{Z}_p$ for $i = 1, \dots, k$.
\STATE Compute $c = H(g, h, \textbf{y}_1, \textbf{y}_2, \textbf{t}_1, \textbf{t}_2)$.
\RETURN $g^{\sum_{i=1}^k \alpha_i s_{1i}} h^{\sum_{i=1}^k \alpha_i s_{2i} + \beta_i s_{3i}} \prod_{i=1}^k y_{1i}^{\alpha_i c + \beta_i s_{1i}} y_{2i}^{c \beta_i} == \prod_{i=1}^k t_{1i}^{\alpha_i} t_{2i}^{\beta_i}$.
\end{algorithmic}
\end{algorithm}

% \begin{algorithm}[t]
%   % \caption{Generate a proof of $(z, y_1, \dots, y_m) = (g^r, g^{x_1} h_1^r, \dots, g^{x_k} h_k^r)$}
%   \caption{$\mathsf{GenPrfWF}(g, h, r, x)$}
%   \label{alg:gen_prf_wf}
% %\hspace*{\algorithmicindent} 
%   \begin{algorithmic}
%     % \STATE \textbf{Def:} 
% %\hspace*{\algorithmicindent} 
%     \STATE Randomly sample $w, v \in \mathbb{Z}_p$.
%     \STATE Compute $u = g^w$, $t = g^{v} h^w$.
%     \STATE Compute $c = H(g, h, z, y, u, t)$.
%     \STATE Compute $s = w - c r$, $s^* = v - c x$.
%     \RETURN $\pi = (c, s, s*)$.
% \end{algorithmic}
% \end{algorithm}

% \begin{algorithm}[t]
%   \caption{$\mathsf{VerPrfWF}(g, h, z, y, \pi)$}
%   \label{alg:ver_prf_wf}
% %\hspace*{\algorithmicindent} 
%   \begin{algorithmic}
% %\hspace*{\algorithmicindent} 
% \STATE Unravel $\pi = (c, s, s^*)$.
%     \STATE Compute $u' = g^s z^c$, $t' = g^{s^*} y^c h^s$.
%     \RETURN $c == H(g, h, z, y, u', t')$.
% \end{algorithmic}
% \end{algorithm}

\begin{algorithm}[t]
  %\caption{$\mathsf{GenPrfWf}(g, h_0, \dots, h_k, z, Y_0, \dots, Y_k, z_1, \dots, z_k, r, x_0, \dots, x_k, q_1, \dots, q_k)$}
  \caption{$\mathsf{GenPrfWf}(g, q, \textbf{h}, z,  \textbf{e}, \textbf{o}, r, \textbf{v}^*, \textbf{s})$}
  \label{alg:gen_prf_wf}
%\hspace*{\algorithmicindent} 
  \begin{algorithmic}
%\hspace*{\algorithmicindent} 
\STATE Randomly Sample $w, x_0, \dots, x_k, x_1', \dots, x_k' \in \mathbb{Z}_p$.
\STATE Compute $u = g^w$, $t_i = g^{x_i} h_i^{w}$ $(\forall i \in [0, k])$, $t_i^* = g^{x_i} q^{x_i'}$ $(\forall i \in [1, k])$.
\STATE Compute $c = H(g, q, \textbf{h}, z, \textbf{e}, \textbf{o}, u, \textbf{t}, \textbf{t}^*)$.
\STATE Compute $y = w - c r$, $y_i = x_i - c v_i$ $(\forall i \in [0, k])$, $y_i' = x_i' - c s_i$ $(\forall i \in [1, k])$, where $\textbf{v}^* = (v_0, \dots, v_k)$ 
\RETURN $\pi = (u, \textbf{t}, \textbf{t}^*, y, \textbf{y}, \textbf{y}')$.
\end{algorithmic}
\end{algorithm}

\begin{algorithm}[t]
  %\caption{$\mathsf{VerPrfWf}(g, h_0, \dots, h_k, z, Y_0, \dots, Y_k, z_1, \dots, z_k, \pi)$}
  \caption{$\mathsf{VerPrfWf}(g, q, \textbf{h}, z, \textbf{e}, \textbf{o},\pi)$}
  \label{alg:ver_prf_wf}
%\hspace*{\algorithmicindent} 
  \begin{algorithmic}
%\hspace*{\algorithmicindent} 
\STATE Unravel $\pi = (u, \textbf{t}, \textbf{t}^*, y, \textbf{y}, \textbf{y}')$.
\STATE Compute $c = H(g, q, \textbf{h}, z, \textbf{e}, \textbf{o}, u, \textbf{t}, \textbf{t}^*)$.
\STATE Randomly sample $\alpha, \beta_i (i \in [0,k])$, $\gamma_i (i \in [1,k]) \in \mathbb{Z}_p$.
\RETURN $u^{\alpha} \prod_{i=0}^k t_i^{\beta_i} \prod_{i=1}^k t_i^{*\gamma_i} == g^{\alpha w + \sum_{i=0}^k \beta_i y_i + \sum_{i=1}^k \gamma_i y_i} z^{\alpha c} \prod_{i=0}^k (h_i^{\beta_i y} e_i^{\beta_i c}) q^{\sum_{i=1}^k \gamma_i y_i'}\prod_{i=1}^k o_i^{c \gamma_i}$.
% \STATE Compute $u' = g^s z^c$. 
% \STATE Compute $t_i' = g^{s_i} Y_i^c h_i^s$ $(i = 0, \dots, k)$.
% \STATE Compute $(t_i^*)' = g^{s_i} z_i^c Q^{s_i'}$ $(i = 1, \dots, k)$.
% \STATE return $c == H(g, h_0, \dots, h_k, z, Y_0, \dots, Y_k, z_1, \dots, z_k, u', t_0', \dots, t_k', (t_1^*)', \dots, (t_k^*)')$.
\end{algorithmic}
\end{algorithm}

\ignore{
\subsection{A detailed analysis of $\mathsf{EIFFeL}$} \label{subsec:eiffel-analysis}

\needcheck{maybe move cost analysis section here?}
% Also, $\mathsf{EIFFeL}$ adopts the secret-shared non-interactive proof (SNIP)~\cite{Corrigan-GibbsB17} for ZKP generation and verification. The cost of proof generation is $O(bmnd)$ field multiplications, where $b$ is the bit length of weight update, for computing Shamir's shares (without check strings) of every bit of every coordinate of the weight update. A 256-bit ECC group exponentiation costs the order of $10^3$ field multiplications \cite{hisil2008twisted}. When $n = 100$ and $m = 10$, this cost is comparable to commitment.
% The cost of proof verification is $O(bnd)$ field multiplications and an additional $O(nmd/\log(md))$ for verification of check strings.
}

\subsection{Chi-square Distribution of Sampling} \label{subsec:chi-square}

% In this section, we provide the chi-square distribution proof and bound the rounding errors occurring in discretizing the normal distribution samples. 

\subsubsection{Proof of Lemma \ref{lem:chi-sq}} \label{subsubsec:lemma-chi-sq-proof}

\begin{proof}[Proof of Lemma \ref{lem:chi-sq}]
% \begin{proof}[Proof]
    Since $\textbf{a}_t$ follows $\mathcal{N}(\textbf{0}, \textbf{I}_d)$, its projection on the direction of $\textbf{u}$, $\langle \textbf{a}_t, \frac{\textbf{u}}{||\textbf{u}||} \rangle$,
    follows $\mathcal{N}(0, 1)$. Therefore, the sum of squares of these inner products for $t \in [1, k]$, 
    \begin{displaymath}
     \frac{1}{||\textbf{u}||_2^2}\sum_{t=1}^k \langle \textbf{a}_t , \textbf{u} \rangle^2,  
    \end{displaymath}
    follows $\chi_k^2$.
\end{proof}

\subsubsection{Proof of Lemma \ref{lem:round}} \label{subsubsec:lemma-round-proof}

\begin{proof}[Proof of Lemma \ref{lem:round}]
% \begin{proof}[Proof]
    We have $|b_{tj} - a_{tj}| \leq 1/2$ for all $t, j$. So $||\textbf{a}_t - \textbf{b}_t||_2 \leq \sqrt{d} / 2$. For every $t$, we have 
    \begin{align*}
        \langle \textbf{a}_t, \textbf{u} \rangle^2 - \langle \textbf{b}_t, \textbf{u} \rangle^2 & = \langle \textbf{a}_t - \textbf{b}_t, \textbf{u} \rangle^2 + 2 \langle \textbf{b}_t, \textbf{u} \rangle  \langle \textbf{a}_t - \textbf{b}_t, \textbf{u} \rangle \\
        & \leq ||\textbf{a}_t - \textbf{b}_t||_2^2 ||\textbf{u}||_2^2 + 2 || \textbf{a}_t - \textbf{b}_t|| \cdot ||\textbf{u}|| \cdot |\langle \textbf{b}_t, \textbf{u} \rangle| \\
        & \leq \frac{1}{4} d B^2 + {\sqrt{d}} \cdot B \cdot |\langle \textbf{b}_t, \textbf{u} \rangle|.
    \end{align*}
    Summing up and using $\sum_{t=1}^k |\langle \textbf{b}_t, \textbf{u} \rangle| \leq \sqrt{k  \sum_{t=1}^k \langle \textbf{b}_t, \textbf{u} \rangle^2 }$, we have
    \begin{align*}
        \sum_{t=1}^k \left( \langle \textbf{a}_t, \textbf{u} \rangle^2 - \langle \textbf{b}_t, \textbf{u} \rangle^2 \right) 
        % & \leq \frac{1}{4} kdB^2 + \sqrt{d} \cdot B \sum_{t=1}^k |\langle \textbf{b}_t, \textbf{u} \rangle| \\
        & \leq \frac{1}{4} kdB^2 + \sqrt{d} \cdot B \sqrt{k  \sum_{t=1}^k \langle \textbf{b}_t, \textbf{u} \rangle^2 } 
         % & \leq \frac{1}{4} kdB^2 + \sqrt{d} \cdot B \sqrt{k  B^2M^2r} \\
         % & = \frac{1}{4} kdB^2 + \sqrt{kdr} \cdot B^2 M
    \end{align*}
    Adding this to the assumption that $\sum_{t=1}^k \langle \textbf{b}_t, \textbf{u} \rangle^2 \leq B^2M^2r$ yields the desired inequality.
\end{proof}

\subsubsection{Proof of Lemma \ref{lem:round_fail}} \label{subsubsec:lemma-round-fail-proof}

\begin{proof}[Proof of Lemma \ref{lem:round_fail}]
% \begin{proof}[Proof]
Continuing with the idea of the proof of Lemma~\ref{lem:round}, we have     
\begin{align*}
        \langle \textbf{a}_t, \textbf{u} \rangle^2 - \langle \textbf{b}_t, \textbf{u} \rangle^2 & = \langle \textbf{a}_t - \textbf{b}_t, \textbf{u} \rangle^2 + 2 \langle \textbf{b}_t, \textbf{u} \rangle  \langle \textbf{a}_t - \textbf{b}_t, \textbf{u} \rangle \\
        & \geq - 2 || \textbf{a}_t - \textbf{b}_t|| \cdot ||\textbf{u}|| \cdot |\langle \textbf{b}_t, \textbf{u} \rangle| \\
        & \geq - {\sqrt{d}} \cdot B \cdot |\langle \textbf{b}_t, \textbf{u} \rangle|.
\end{align*}
Summing up, we have 
    \begin{align*}
        \sum_{t=1}^k \left( \langle \textbf{a}_t, \textbf{u} \rangle^2 - \langle \textbf{b}_t, \textbf{u} \rangle^2 \right) 
        % & \geq - \sqrt{d} \cdot B \sum_{t=1}^k |\langle \textbf{b}_t, \textbf{u} \rangle| \\
        & \geq - \sqrt{d} \cdot B \sqrt{k  \sum_{t=1}^k \langle \textbf{b}_t, \textbf{u} \rangle^2 }.
    \end{align*}
After moving $\sum_{t=1}^k \langle  \langle \textbf{b}_t, \textbf{u} \rangle^2 $ to the right and completing the square, we get
\begin{align*}
    \sqrt{ \sum_{t=1}^k \langle \textbf{b}_t, \textbf{u} \rangle^2 } &\leq \sqrt{\sum_{t=1}^k \langle \textbf{a}_t, \textbf{u} \rangle^2 + \left(\frac{B\sqrt{kd}}{2}\right)^2 } + \frac{B\sqrt{kd}}{2} \\
    & \leq \sqrt{\sum_{t=1}^k \langle \textbf{a}_t, \textbf{u}\rangle^2} + B \sqrt{kd} \\ 
    & \leq \sqrt{B_0} + B \sqrt{kd} \\
    & = BM \left( \sqrt{r_{k,\epsilon}} + \frac{3 \sqrt{kd}}{2M} \right).
\end{align*}
After squaring both sides and dividing by $|| \textbf{u} ||_2^2$, we obtain the desired inequality.
\end{proof}

\subsection{The Complete Security Proof} \label{subsec:complete-proof}

\subsubsection{Proof of Lemma \ref{lem:pass}} \label{subsubsec:lemma-pass-proof}

%\begin{proof}[Proof of Lemma \ref{lem:pass}]
\begin{proof}[Proof]
We have $||\textbf{u}_i||_2 \leq B$. By Lemma~\ref{lem:chi-sq}, the probability that 
\begin{displaymath} \label{eq:chisquare-prob}
        \sum_{t=1}^k \langle \textbf{b}_t, \textbf{u}_i \rangle^2 \leq B^2M^2\gamma_{k, \epsilon}
\end{displaymath}
is at least $1 - \epsilon$.
By Lemma~\ref{lem:round}, the probability that 
\begin{displaymath} 
\label{eq:lem_sum_bound}
    \sum_{t=1}^k \langle \textbf{a}_t, \textbf{u}_i \rangle^2 \leq B_0
\end{displaymath} is at least $1 - \epsilon$. If Eqn~\ref{eq:lem_sum_bound} holds, $\mathcal{C}_i$ can produce a proof which passes the integrity check.
\end{proof}

\subsubsection{Proof of Lemma \ref{lem:break}} \label{subsubsec:lemma-break-proof}

\begin{proof}[Proof of Lemma~\ref{lem:break}]
% \begin{proof}[Proof]
    The function $\mathsf{VerPrfWf}$ and the large sampling space $\mathbb{Z}_p$ on each coordinate ensures that $\mathcal{C}_i$ must be able to efficiently respond to any $\textbf{a}_0$ by producing $v_0$ and $r$ that satisfies $g^{v_0} h_0^{r} = e_0$. The function $\mathsf{VerCrt}$ ensures that $e_0 = \prod_{l=1}^d y_{il}^{a_{0l}}$. That is, 
    \begin{equation}\label{eq:wf}
        g^{v_0} h_0^{r} = \prod_{l=1}^d y_{il}^{a_{0l}}.
    \end{equation} 
    If we change $\textbf{a}_0$ to $\textbf{a}_0'$, $\mathcal{C}_i$ produces $v_0'$ and $r'$ that satisfies $g^{v_0'} (h_0')^r = \prod_{l=1}^d y_{il}^{a_{0l}'}$. Therefore, 
    \begin{displaymath}
        g^{v_0' - v_0} \prod_{l=1}^d w_l^{a_{0l}' r' - a_{0l} r} = \prod_{l=1}^d y_{il}^{a_{0l}' - a_{0l}}.
    \end{displaymath}
    For each $l$, by setting $a_{0j}'= a_{0j} + \delta_{lj}$ where $\delta_{lj} = 1$ if $l=j$, $\delta_{lj} = 0$ if $l\neq j$, we get that each $y_{il}$ can be expressed into the form 
    \begin{displaymath}
        y_{il} = g^{\alpha_l} \prod_{j=1}^d w_j^{\beta_{lj}}.
    \end{displaymath}
    We would like to have $\beta_{lj}=0$ whenever $l \neq j$. Suppose not and without loss of generality, $\beta_{12} \neq 0$. 
    Equation~\ref{eq:wf} becomes
    \begin{displaymath}
        g^{v_0} \prod_l w_l^{r a_{0l}} = g^{\sum_l a_{0l} \alpha_l} \prod_l w_l^{ \sum_j a_{0j}\beta_{jl}}.
    \end{displaymath}
    If we change $\textbf{a}_0$ to $\textbf{a}_0'$ where $a_{01}' = a_{01} + 1$, $a_{0l}' = a_{0l}$ for $l \geq 2$ and $\mathcal{C}_i$ produces $v_0'$ and $r'$, we get 
    \begin{displaymath}
    g^{v_0'} \prod_l w_l^{r' a_{0l}'} = g^{\sum_l a_{0l}' \alpha_l} \prod_l w_l^{\sum_j a_{0j}' \beta_{jl}}.
    \end{displaymath}
    Dividing these two inequalities, we get 
    \begin{displaymath}
    g^{v_0'-v_0} \prod_l w_l^{r'a_{0l}' - r a_{0l}} = g^{\alpha_1}  \prod_l w_l^{\beta_{1l}}.
    \end{displaymath}
    Because $g, w_1, \dots, w_d$ are independent, we must have $v_0' - v_0 = \alpha_1$, $r' a_{0l}' - r a_{0l} = \beta_{1l}$. So $(r'-r)a_{01} + r' = \beta_{11}$, $(r'-r)a_{0l} = \beta_{1l}$ for $l \geq 2$. If $r' \neq r$, then we must have $a_{02}^{-1} a_{03} = \beta_{12}^{-1} \beta_{13}$. So whenever $a_{02}^{-1} a_{03} \neq \beta_{12}^{-1} \beta_{13}$, we must have $r' = r$, and then $r' = \beta_{11}$, so
    \begin{displaymath}
        r' a_{0l}' = \beta_{11} a_{0l}' = \sum_j a_{0j}' \beta_{jl}.
    \end{displaymath}
    for any $l$. So $\beta_{11} = \beta_{ll}$ and $\beta_{jl}=0 $  whenever $j \neq l$. This is a contradiction. 

    We have concluded that $\beta_{lj} = 0$ whenever $l \neq j$. So 
    \begin{displaymath}
        g^{v_0} \prod_l w_l^{r a_{0l}} = g^{\sum_l a_{0l}\alpha_l} \prod_l w_l^{a_{0l} \beta_{ll}}.
    \end{displaymath}
    Therefore,  $v_0 = \sum_l a_{0l} \alpha_l$ and $r = \beta_{ll}$. This ensures that client $\mathcal{C}_i$'s commitment must satisfy $y_{il} = g^{\alpha_l} w_l^{r}$, which is exactly the required form in the protocol. 

    So far, we have shown well-formedness of $\textbf{y}_i$. To pass the integrity check, client $\mathcal{C}_i$ must submit correct computations of $e_t$, submit $o_t, o_t'$ of the correct form, and submit boundedness proofs for each inner product and final sum. So $\textbf{u}_i$ must satisfy equation~\ref{eq:lem_sum_bound}.
\end{proof}

\subsubsection{Proof of Lemma \ref{lem:fail}} \label{subsubsec:lemma-fail-proof}

\begin{proof}
By Lemma~\ref{lem:round_fail},
the probability that Eqn~\ref{eq:lem_sum_bound} holds is at most $\mathrm{Pr}_{x \sim \chi_k^2}[x < \frac{1}{D(\textbf{u}_i)^2} \left( \sqrt{\gamma_{k,\epsilon}} + \frac{3 \sqrt{kd}}{2M} \right)^2]$. If Eqn~\ref{eq:lem_sum_bound} does not hold, by Lemma~\ref{lem:break}, the probability that $\mathcal{C}_i$ produces a valid proof is $\mathrm{negl}(\kappa)$. The sum of these two probabilities is $F_{k, \epsilon, d, M}(D(\textbf{u}_i))$.
\end{proof}

\subsubsection{Proof of Theorem \ref{theorem:security}} \label{subsubsec:theorem-proof}
\red{add a more formal proof of this Theorem}
%\begin{proof}[Proof of Theorem~\ref{theorem:security}]
\begin{proof}[Proof]
    Input integrity is already proved in Lemma~\ref{lem:output}. We now prove input privacy. Given an adversary $\mathcal{A}$ that consists of the malicious server and the malicious clients $\mathcal{C}_M$ attacking the real interaction, we define a simulator $\mathcal{S}$ as required. 

    $\mathcal{S}$ is defined by modifying $\mathcal{A}$ at each step when the server or the malicious clients $\mathcal{C}_M$ read inputs from one of the honest clients $\mathcal{C}_H$. In the ideal functionality $\mathcal{F}$, the honest clients $\mathcal{C}_{\mathcal{H}}$ hold values $\{\textbf{u}_i'\}_{\mathcal{C}_i \in \mathcal{C}_H}$ that is randomly picked from 
    \begin{displaymath}
        \{ \{\textbf{u}_i''\}_{\mathcal{C}_i \in \mathcal{C}_H} : \sum_{\mathcal{C}_i \in \mathcal{C}_H} \textbf{u}_i'' = \mathcal{U}_{\mathcal{H}}, \forall i ~ ||\textbf{u}_i''|| \leq B\}.
    \end{displaymath}
    In $\mathcal{S}$, the client $\mathcal{C}_i \in \mathcal{C}_H$, uses $\textbf{u}_i'$ and random value $r_i'$ as its weight update to make commitments. After receiving the samples $\textbf{A}$ from the server, the client $\mathcal{C}_i \in \mathcal{C}_H$, sends a proof to the server if Eqn~\ref{eq:lem_sum_bound} holds, and aborts if Eqn~\ref{eq:lem_sum_bound} does not hold. By Lemma~\ref{lem:pass}, the probability that one of the clients in $\mathcal{C}_H$ fails in $\mathcal{A}$ or $\mathcal{S}$ is $\mathrm{negl}(\kappa)$. 
    %\needcheck{conflicting notation: the simulation and the server both use $\mathcal{S}$} 
    %% wyc: have removed the notation of malicious server $\mathcal{S}$, so only the simulator uses this notation
    At the aggregation step, in both $\mathcal{A}$ and $\mathcal{S}$, the property of Shamir's sharing ensures that the server can only infer the sum of the secrets $\sum_{\mathcal{C}_i \in \mathcal{C}_H} {r}_i$, $\sum_{\mathcal{C}_i \in \mathcal{C}_H} r_i'$ respectively. The only information that the server can infer from this sum is $\mathcal{U}_H$. 

    Therefore, if Eqn~\ref{eq:lem_sum_bound} holds for all $\mathcal{C}_i \in \mathcal{C}_H$ in both $\mathcal{A}$ and $\mathcal{S}$, the colluding party of the server and malicious clients $\mathcal{C}_{M}$ cannot infer anything from the proofs generated by $\mathcal{C}_H$ except $\mathcal{U}_H$, which means that 
    \begin{displaymath}
         |\mathrm{Pr} [\mathrm{Real}_{\Pi, \mathcal{A}} (\{\textbf{u}_{\mathcal{C}_H}\}) = 1] - \mathrm{Pr}[\mathrm{Ideal}_{\mathcal{F}, \mathcal{S}} (\mathcal{U}_H) = 1]| \leq \mathrm{negl}(\kappa).
    \end{displaymath}
    This inequality still holds after counting in the probability $\mathrm{negl}(\kappa)$ that one of the clients in $\mathcal{C}_H$ fails the check. 
    % we conclude that
    % \begin{displaymath}
    %     |\mathrm{Pr} [\mathrm{Real}_{\Pi, \mathcal{A}} (\{\textbf{u}_{\mathcal{C}_H}\}) = 1] - \mathrm{Pr}[\mathrm{Ideal}_{\mathcal{F}, \mathcal{S}} (\mathcal{U}_H) = 1]| \leq \mathrm{negl}(\kappa).
    % \end{displaymath}
\end{proof}

\begin{figure}[t]
    \centering
    {\includegraphics[width=0.35\textwidth]{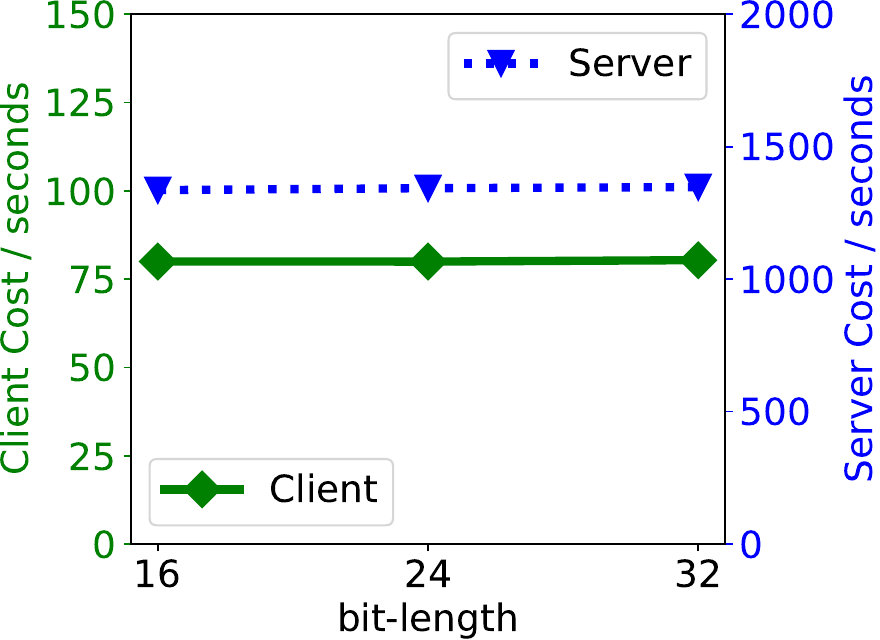} }
    \caption{Cost comparison w.r.t. bit-length}
    \label{fig:bits}
\end{figure}

\subsection{The Implementation Detail of \eiffel{}} \label{appendix:eiffel}

Since \eiffel{} is not open-sourced, we implement it from scratch for a fair comparison. Two differences exist between our \eiffel{} experiments and those in the original paper. 

First, we add bound checks for every coordinate of the model updates, use the information-secure VSSS and the multiplicative homogeneity of Shamir's share to compute shares of the sum of squares, and use the batch checking to verify the check strings of VSSS, as discussed in Section~\ref{sec:analysis}.

% 2. We use the information-secure VSSS \cite{pedersen2001non} to share the weight updates. This is necessary to protect the weight updates, as discussed in Section~\ref{sec:analysis}.

% VSS in the original paper is not secure because weight updates are small. Need to use information-secure \cite{pedersen2001non}.
% Client $i$ shares $x_{il}$ for $l \in [d]$ with VSS. Note that since $x_{il}$ is small, it can be easily computed from $g^{x_{il}}$. so the Feldman VSS \cite{feldman1987practical} involving $g^{x_{il}}$ cannot be used. Instead, we have to use an information-theoretic secure alternative \cite{pedersen2001non}, which involves $2m+1$ group exponentiations for Byzantine tolerance of $m$ malicious clients (ignoring the cost of the small power $g^{x_{il}}$). 

% 3. We use the multiplicative homogeneity of Shamir's share to compute shares of sum of squares at the cost of requiring that $m < (n-1)/4$. This is discussed in \cite[Section 11.1]{roy2022eiffel}. The corresponding cost is $O(d)$ per sum of squares. In comparison, the polynomial interpolation approach in \cite[Section 11.1]{roy2022eiffel} is actually $O(d^2)$ per sum of squares, because one needs to compute $d$ values of polynomials of degree $d$, even if the Lagrange coefficients are precomputed.
% which is too costly. For $l_2$ norm bound, we don't need them. Just use muliplicity of Shamir Share.

Second, we use $3m+1$ shares, instead of $n$ shares, to perform robust reconstruction~\cite{gao2003new} that tolerates $m$ errors. This saves the cost of robust reconstruction by a factor of $n^2 / (3m+1)^2$ compared to their original implementation. 

% 5. We use batch checking to verify check strings of VSSS, as discussed in Section~\ref{sec:analysis}.
% In order to verify that $u_i = \prod_{j=1}^t v_{ij}^{a_{ij}}$ for all $i \in [1, s]$, we randomly sample $\alpha_i \in \mathbb{Z}_p$, $i \in [1,s]$ and verify that $\prod_{i=1}^s u_i^{\alpha_i} = \prod_{i=1}^s \prod_{j=1}^t v_{ij}^{\alpha_i a_{ij}}$. This saves the cost of check string verification by a factor of $O(\log(bd))$.

\subsection{Effects of bit-length of weight updates} \label{appendix:bits}

We compare the effect of the integer bit-length that encodes clients' model updates on the client computational time and server computational time. We fix the number of parameters $d = 1$M, the number of samples $k = 1$K, the number of clients $n=100$, the maximum number of malicious clients $m = 10$, and vary bit-length in $\{16, 24, 32\}$.
Figure~\ref{fig:bits} shows the experimental results. We can observe that the effect of the bit-length on the cost is small.
